# Supplementary material for: Modelling M/M/R-JSQ-PS sojourn time distribution for Ultra-Reliable Low Latency Communication services
Source: arXiv:2210.17227 source file (2022-12-22)
Supplement: Supplementary file 1 [file appendix.tex]

\appendices

\section{Errors for increasing
reliabilities}
\label{app:percentile-errors}

\setcounter{figure}{13}    
\setcounter{equation}{26}    

Fig.~\ref{fig:all-percentile-sojourn-errors}
shows the error for the best
approximation A-F
from the 99\textsuperscript{th} up to
the 99.999\textsuperscript{th} percentile of the
sojourn time. The sojourn time error is unitless,
and it illustrates the increasing error as
$\rho$ approaches $1$, so as the increasing oscilacions of
the error for higher reliabilities, even with
mid values of the number of CPUs like $R=4$ --
as explained in
Section~\ref{sec:behaviour-high-reliabilities}.
% Section~8.

\begin{figure}[ht!]
    \centering

    \subfloat[]{\includegraphics[width=0.57\columnwidth]{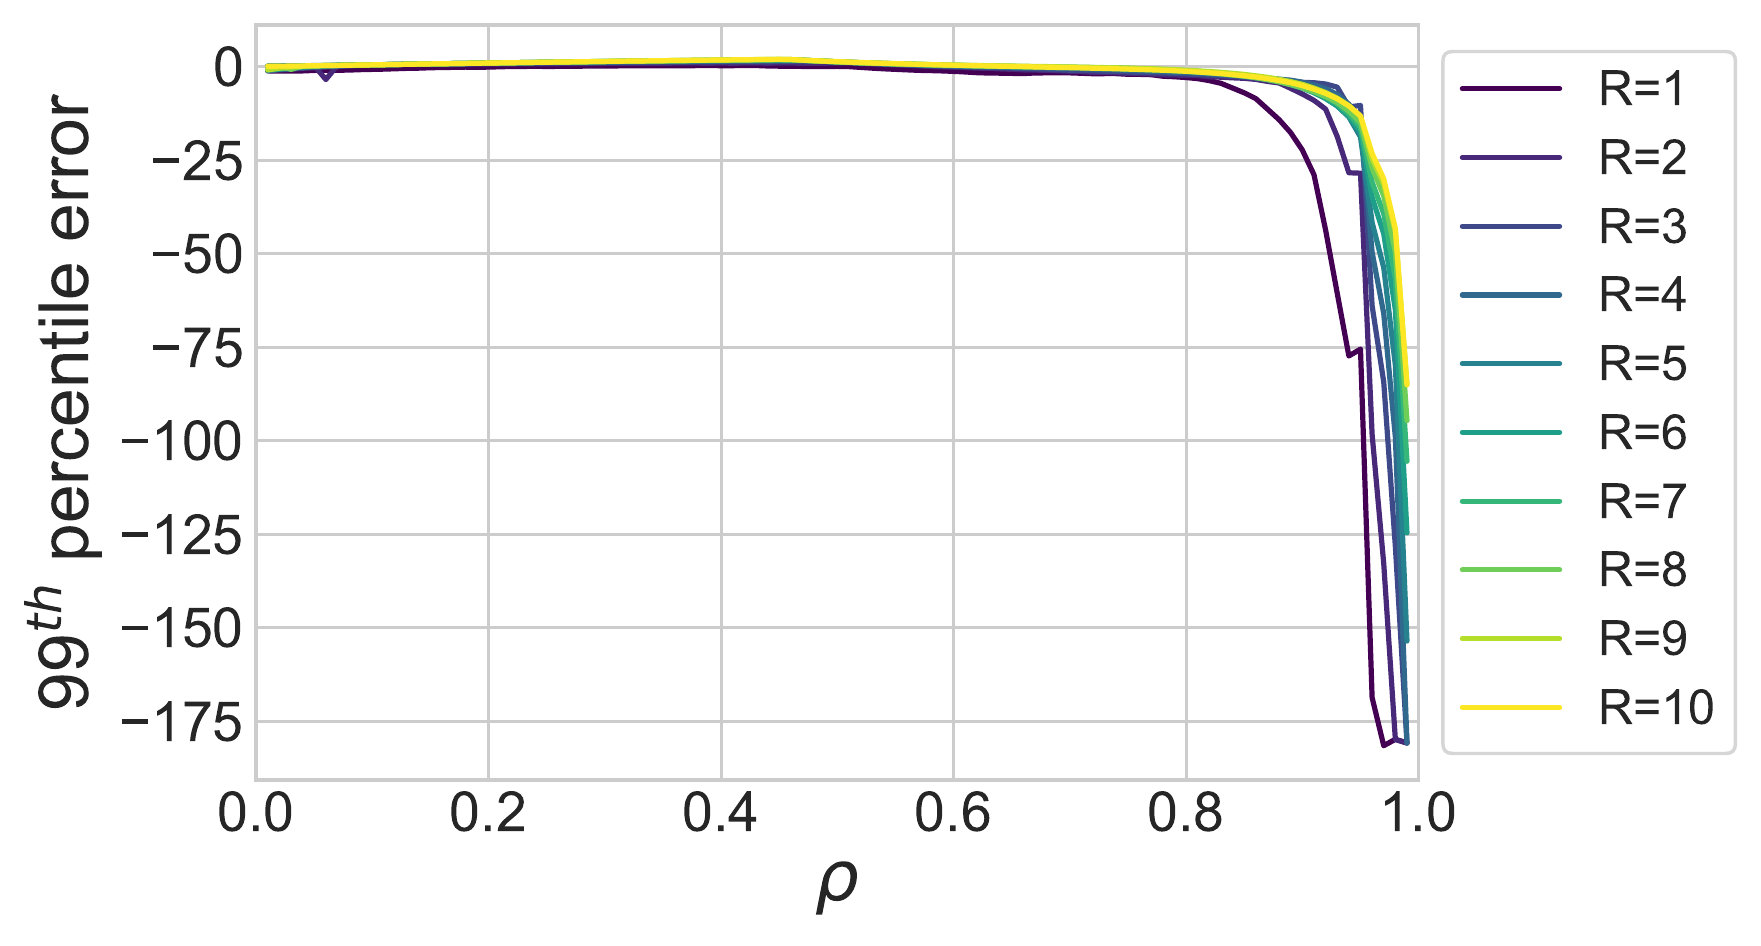}} \\
    \subfloat[]{\includegraphics[width=0.57\columnwidth]{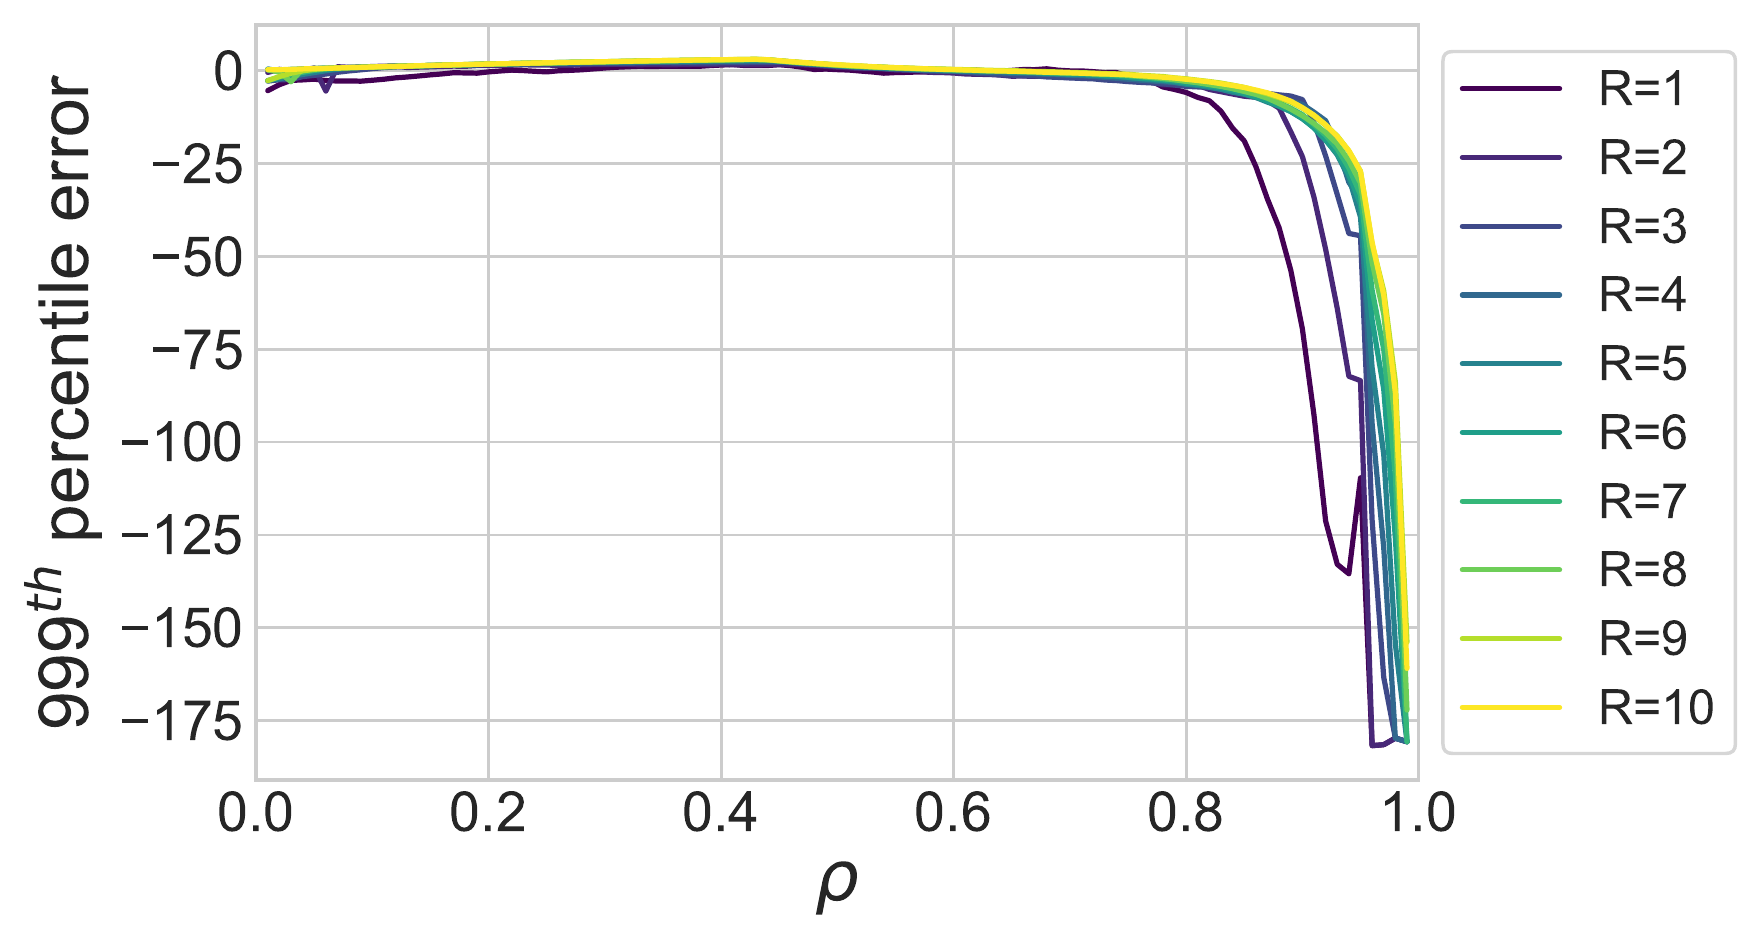}} \\
    \subfloat[]{\includegraphics[width=0.57\columnwidth]{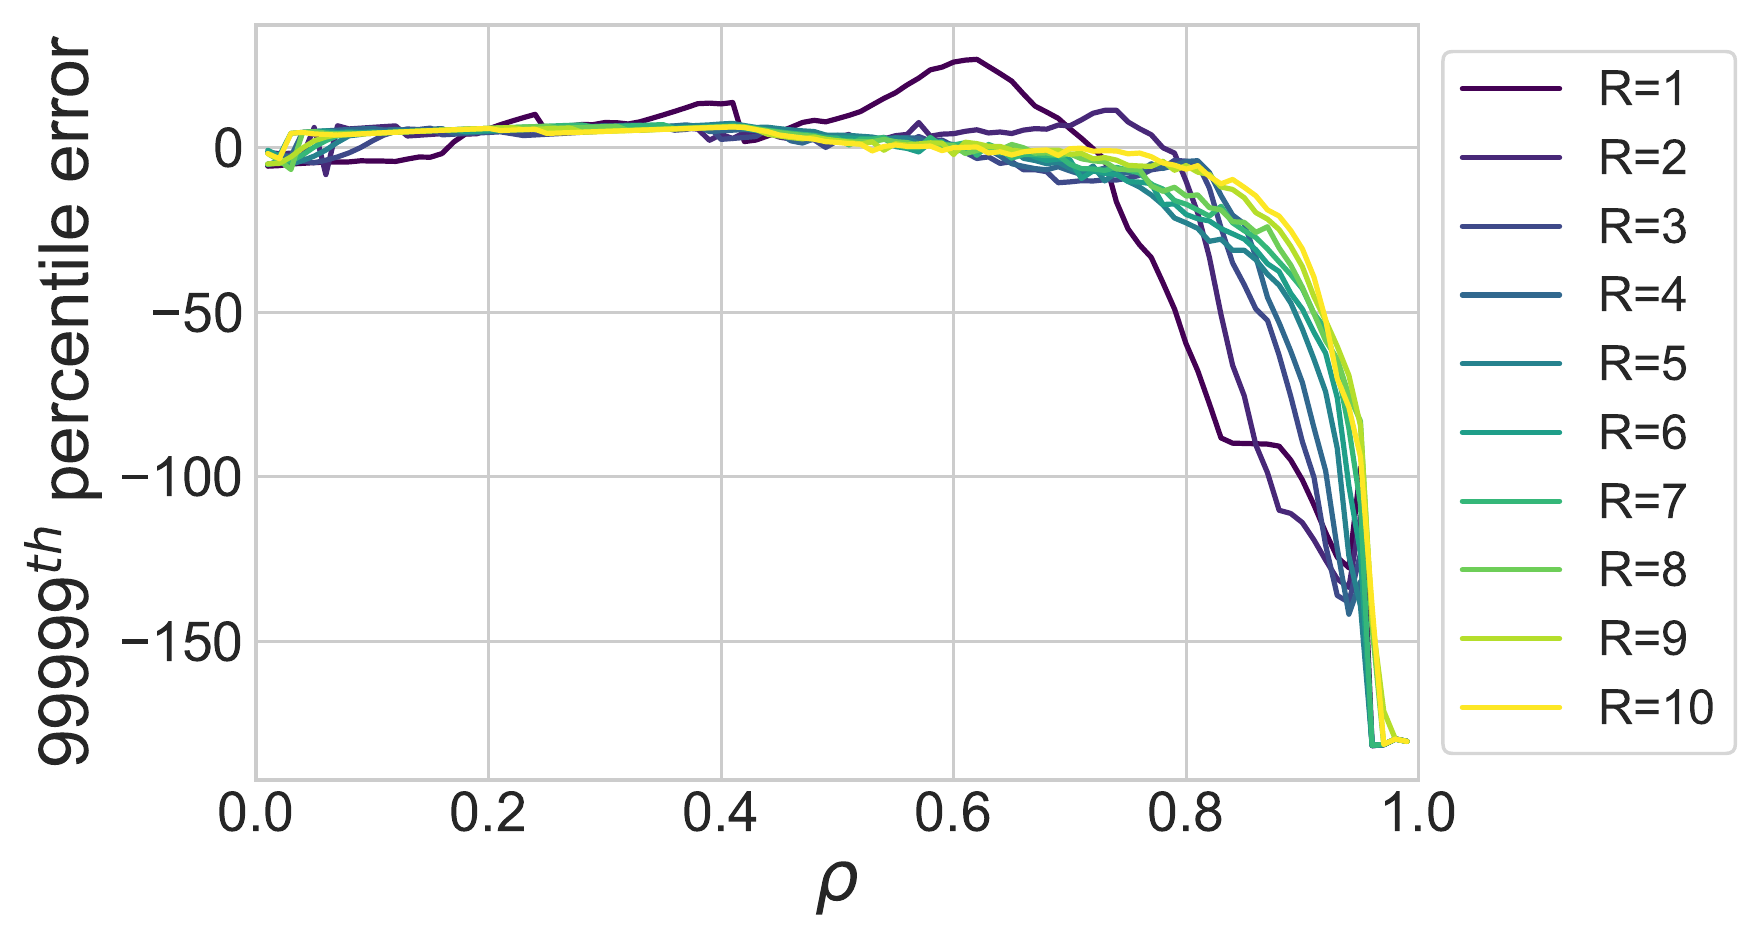}} \\

    \caption{The best method error for the
        99\textsuperscript{th},
        99.9\textsuperscript{th}, and
        99.999\textsuperscript{th}
        percentile the sojourn time.
 Positive/negative mean over/under-estimation, respectively.
    }
    \label{fig:all-percentile-sojourn-errors}
\end{figure}

\section{Getting \texttt{sojourn\_percentile($\eta',R'$)}}
\label{app:sojourn-percentile}

We provide an open-source implementation\footnote{\url{https://github.com/geraintpalmer/mmr-jsq-ps/}}
of the proposed approximation methods~A-F.
Every method is implemented in Python and
yields the sojourn time CDF for a given
number of CPUs $R$. Additionally, it is possible
to specify the truncation limits for the maximum number
of customers considered at each CPU $L_1$, and the
maximum number of customers at the system $L_2$.

In order to obtain the result of the
\texttt{sojourn\_percentile($\eta',R'$)}
function used inside
Algorithm~\ref{alg:scaling},
% Algorithm~1,
we first compute the load $\rho$ given
a number of CPUs $R'$, and the arrival and
service rates $\Lambda,\mu$; respectively.
Second, we check
Fig.~\ref{fig:bestperforming}
% Fig.~7
to know 
which is the best method for the given $(\rho,R')$ tuple,
e.g., method-A.
Third, we create an instance of method-A invoking
\texttt{jsq.MethodA($\Lambda,\mu,R,L_1,L_2, \{t_0,t_1,\ldots\}$)},
with $\{t_0,t_1,\ldots\}$ being the discrete time points
at which we compute the CDF.
Then, we obtain the CDF of method-A
by accessing property \texttt{sojourn\_time\_cdf} of the method instance.
This property holds a vector
$\{P_0,P_1,\ldots\}$ that represents the
CDF computed by method-A. In particular, each element
represents $P_i=\mathbb{P}(T\leq t_i)$.
Finally, we obtain the $\eta'$ percentile of the sojourn time as
\begin{equation}
    t^{\eta'}=\argmin\{t_i: \mathbb{P}(T\leq t_i)>\eta'\}
\end{equation}

\section{Considered $\mu$ for autonomous driving}
\label{app:deriving-mu}
The scaling experiments presented in
Section~\ref{subsec:example}
% Section~9.1
consider an autonomous driving service, namely, an infrastructure
assisted environment perception service~\cite{5g-americas}.
Vehicles send an \mbox{H.265/HEVC} video stream that is processed
in a remote server (modelled as an M/M/R-JSQ-PS system)
to detect road events and inform the vehicle.

The vehicles video stream $\Lambda$ is expressed as frames/sec (fps), and
is processed at a rate of $\mu$ fps in the server hosting
the autonomous driving service. For the experiments in
Section~\ref{subsec:example}
% Section~9.1
we take into consideration the time
that it takes to decode the video stream, and the time it takes for
a Convolutional Neural Network (CNN) to detect events in a video frame.
According to~\cite{decoding,cnn-detection} an Intel Xeon family CPU manages
decode an HEVC video frame in 8~ms, and takes 0.37~ms
to detect a road event in a video frame.
Hence a single CPU within the considered M/M/R-JSQ-PS system
offers a rate of $\mu=\tfrac{10^3}{8.37}$~fps for the considered
infrastructure assisted environment perception service.
Such value of $\mu$ is the one we used in the experiments presented
in
Section~\ref{subsec:example}.
% Section~9.1.
